# Supplementary material for: Decoherence of Coupled Flip-Flop Qubits Due to Charge Noise
Source: arXiv:2104.07485 source file (2021-04-15)
Supplement: Supplementary file 1 [file appendix_effective_ham.tex]

\begin{equation}
    H_0=\left( \begin{array}{cccccc}
          2E_0 &              0 &              0 & V_{dd}z_{31}^2 & 0 & 0                  \\
             0 &        E_0+E_1 & V_{dd}z_{31}^2 &              0 & 0 & V_{dd}z_{31}z_{10} \\
             0 & V_{dd}z_{31}^2 &        E_0+E_1 &              0 & V_{dd}z_{31}z_{10} & 0 \\
V_{dd}z_{31}^2 &              0 &                &              2E_1 & 0 & 0                  \\
             0 &              0 & V_{dd}z_{31}z_{10} & 0 & E_0+E_2 & V_{dd}z_{10}^2 \\
             0 & V_{dd}z_{31}z_{10} & 0 & 0 & V_{dd}z_{10}^2 & E_0 + E_2
     \end{array}\right)
 \end{equation}
