# Supplementary material for: Decoherence of Coupled Flip-Flop Qubits Due to Charge Noise
Source: arXiv:2104.07485 source file (2021-04-15)
Supplement: Supplementary file 2 [file appendix_rotation_matrix.tex]

\begin{equation}
    R=\frac{1}{\sqrt{2}}\left(
    \begin{array}{cccccc}
         \sqrt{2}\cos(\theta/2)&0&0&-\sqrt{2}\sin(\theta/2)&0&0\\
         0&\cos(\phi_+/2)& \cos(\phi_-/2)&0&-\sin(\phi_+/2)&-\sin(\phi_-/2)\\
         0&\cos(\phi_+/2)&-\cos(\phi_-/2)&0&-\sin(\phi_+/2)& \sin(\phi_-/2)\\
         \sqrt{2}\sin(\theta/2)&0&0&\sqrt{2}\sin(\theta/2)&0&0\\
         0&\sin(\phi_+/2)& \sin(\phi_-/2)&0& \cos(\phi_+/2)& \cos(\phi_-/2)\\
         0&\sin(\phi_+/2)&-\sin(\phi_-/2)&0& \cos(\phi_+/2)&-\cos(\phi_-/2)
     \end{array}\right)
 \end{equation}
